# Supplementary material for: Knowledge Consultation for Semi-Supervised Semantic Segmentation
Source: arXiv:2503.10693 source file (2025-03-12)
Supplement: Supplementary file 1 [file Supplementary.tex]

% Ensure single-column format for supplementary material
% Ensure single-column format for supplementary material
\onecolumn  
\clearpage  

% Title Formatting
\begin{center}
    {\fontsize{14pt}{16pt} \selectfont \textbf{Knowledge Consultation for Semi-Supervised Semantic Segmentation}}\\[1.5ex]
    {\large Supplementary Material}
\end{center}

% % Adjust spacing to prevent unwanted blank pages
% \vspace{1ex}  % Add small vertical space before section heading

% Reset figure counter to start from 'a'
\setcounter{figure}{0}  
  % Use a, b, c, d for figures

% Adjust spacing to prevent unwanted blank pages
\vspace{1ex}  % Add small vertical space before section heading

% Force the Section Title to Stay with the Page Number
\FloatBarrier
\section*{A. More Visualizations (Figure \ref{fig:gt_pascal} \& \ref{fig:gt_city} \& \ref{fig:gt_pascal_u2pl_1} \& \ref{fig:gt_pascal_u2pl_2})}
\FloatBarrier

% Reduce extra space before figure
\vspace{-2ex}  

    % First Image (Figure 5) - Ensure it appears directly under Section A
    \begin{figure}[H]  % [H] forces immediate placement
        \centering
        \includegraphics[width=0.65\textwidth]{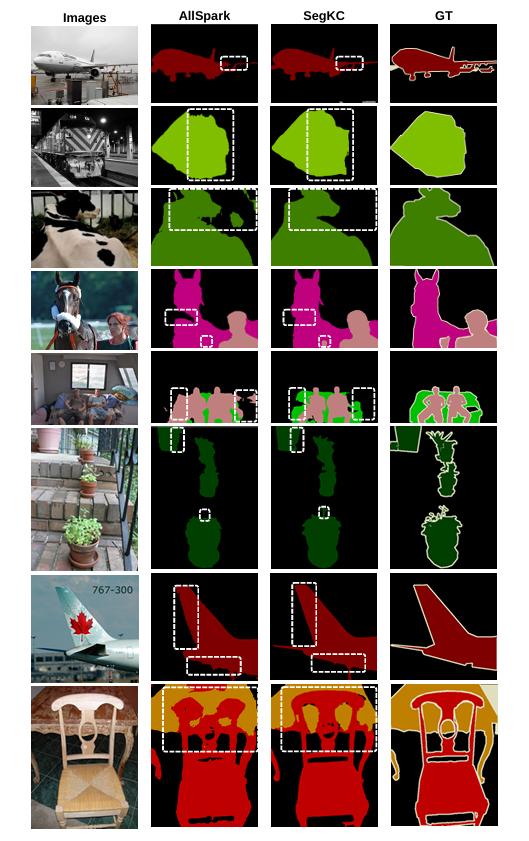}  % Reduce size slightly
        \caption{More visualization of Qualitative comparison on the original Pascal VOC in Figure~\ref{fig:qualitative_pascal}}
        \label{fig:gt_pascal}
    \end{figure}

% Remove excessive space before next figure
\vspace{-1ex}

% Force the second image (Figure 6) onto a separate new page
\clearpage
\begin{figure}[p]
    \centering
    \includegraphics[width=0.95\textwidth]{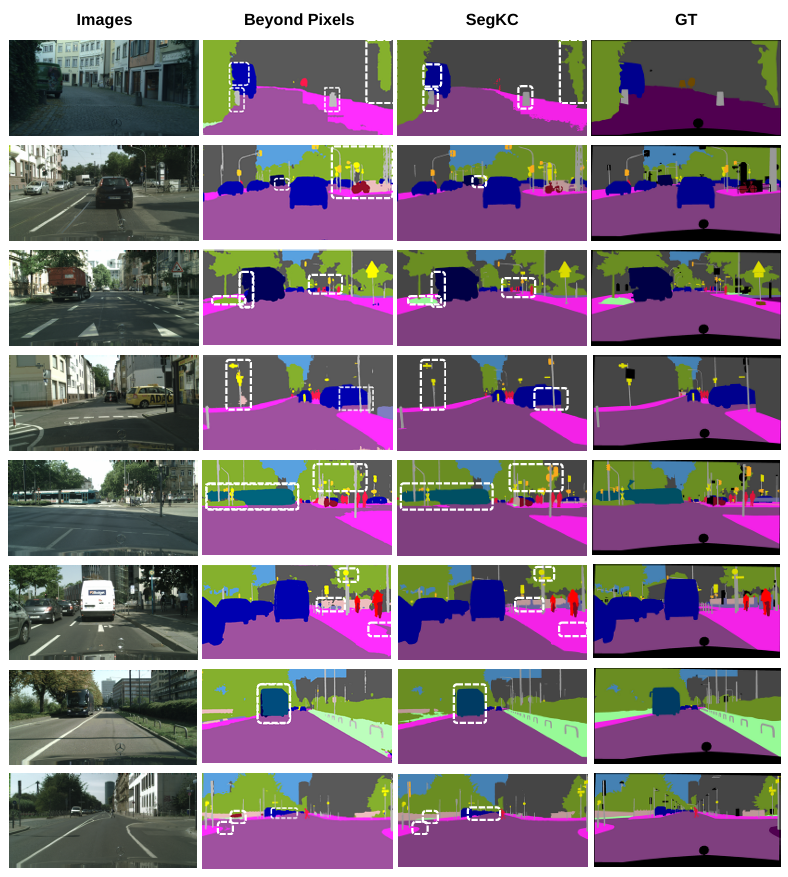}
    \caption{More visualization of Qualitative comparison on the Cityscapes in Figure~\ref{fig:qualitative_cityscapes}}
    \label{fig:gt_city}
\end{figure}

%     % First Image (Figure 5) - Ensure it appears directly under Section A
%     \begin{figure}[H]  % [H] forces immediate placement
%         \centering
%         \includegraphics[width=0.85\textwidth]{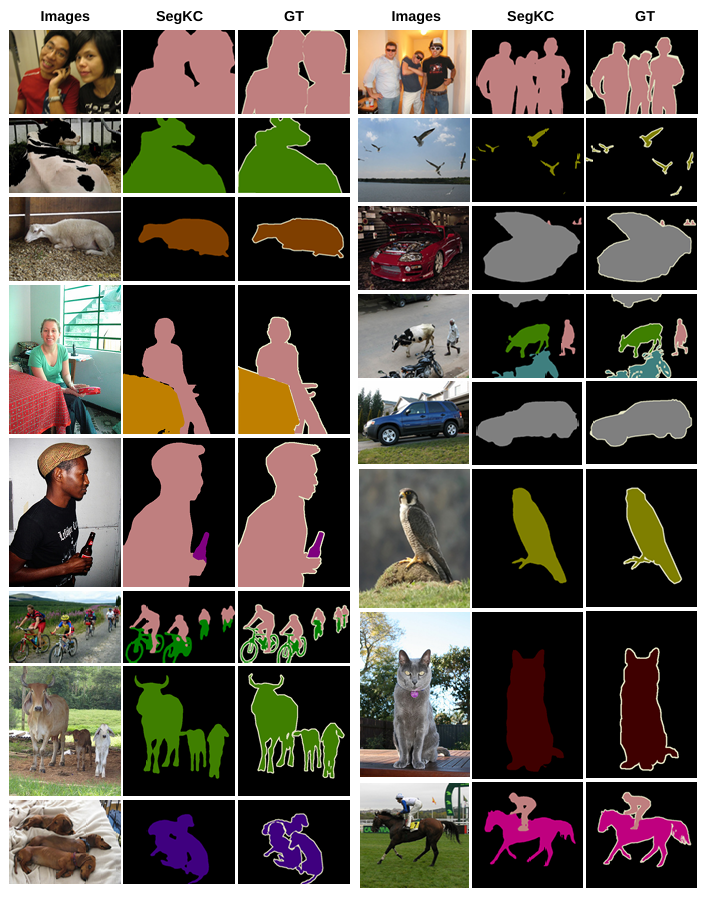}  % Reduce size slightly
%         \caption{GT Pascal U2PL - Case 1}
%         \label{fig:gt_pascal_u2pl_1}
%     \end{figure}
% \end{minipage}

% Remove excessive space before next figure
\vspace{-1ex}

% Force the second image (Figure 6) onto a separate new page
\clearpage
\begin{figure}[p]
    \centering
    \includegraphics[width=0.95\textwidth]{figure/GT_pascal_u2pl_1.png}
    \caption{More visualization of Qualitative comparison of SegKC on Pascal $U^2PL$ split (part 1) which corresponds to the result of Table~\ref{tab:pascal_augmented}}
    \label{fig:gt_pascal_u2pl_1}
\end{figure}

% Remove excessive space before next figure
\vspace{-1ex}

% Force the second image (Figure 6) onto a separate new page
\clearpage
\begin{figure}[p]
    \centering
    \includegraphics[width=0.95\textwidth]{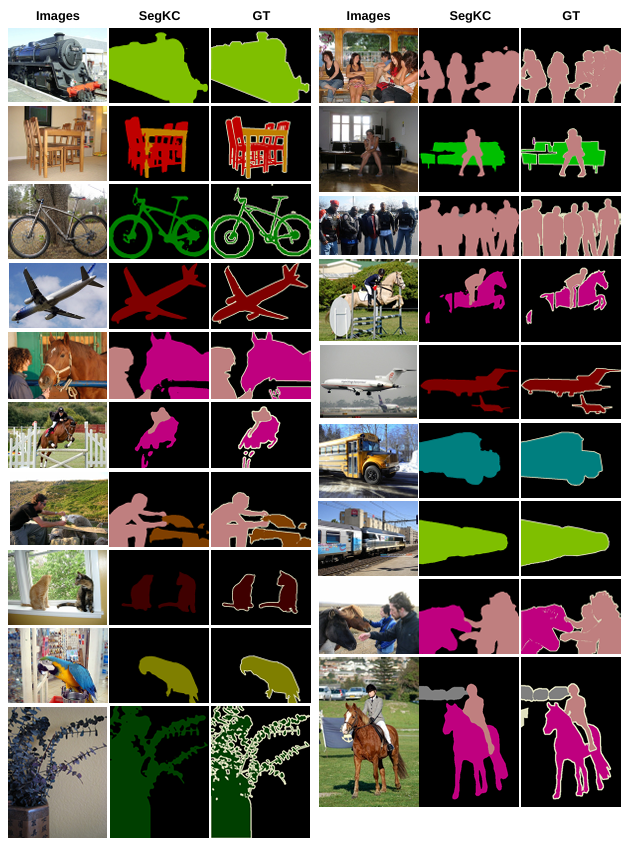}
    \caption{More visualization of Qualitative comparison of SegKC on Pascal $U^2PL$ split (part 2) which corresponds to the result of Table~\ref{tab:pascal_augmented}}
    \label{fig:gt_pascal_u2pl_2}
\end{figure}
